# Supplementary material for: MemArena: An Ego-Centric Benchmark for On-Device Agentic Personal Memory Assistants at Scale
Source: arXiv:2608.02613 source file (2026-10-02)
Supplement: Supplementary file 1 [file appendix_L_body.tex]

\multirow{5}{*}{Vanilla}
  & Qwen3-0.6B     & 44.4{\scriptsize$\pm$0.5} & 10.3{\scriptsize$\pm$0.3} & 15.7{\scriptsize$\pm$0.3} & 7.0{\scriptsize$\pm$0.3} & 58.8{\scriptsize$\pm$0.0} & 0.0{\scriptsize$\pm$0.0} & 22.7{\scriptsize$\pm$0.1} \\

  & Llama-3.2-3B   & 58.6{\scriptsize$\pm$2.3} & 3.2{\scriptsize$\pm$0.3} & 27.8{\scriptsize$\pm$0.2} & 2.9{\scriptsize$\pm$0.8} & 58.4{\scriptsize$\pm$0.3} & 0.0{\scriptsize$\pm$0.0} & 25.2{\scriptsize$\pm$0.3} \\

  & Mistral-7B     & 54.7{\scriptsize$\pm$0.6} & 2.2{\scriptsize$\pm$0.3} & 37.3{\scriptsize$\pm$0.8} & 3.2{\scriptsize$\pm$0.3} & 56.7{\scriptsize$\pm$0.3} & 0.0{\scriptsize$\pm$0.0} & 25.7{\scriptsize$\pm$0.1} \\

  & Qwen3-8B       & 55.7{\scriptsize$\pm$0.6} & 1.8{\scriptsize$\pm$0.0} & 26.6{\scriptsize$\pm$0.3} & 2.7{\scriptsize$\pm$0.7} & 58.8{\scriptsize$\pm$0.0} & 0.0{\scriptsize$\pm$0.0} & 24.3{\scriptsize$\pm$0.2} \\

  & Qwen3-32B      & 66.7{\scriptsize$\pm$0.5} & 1.8{\scriptsize$\pm$0.0} & 28.6{\scriptsize$\pm$0.8} & 1.1{\scriptsize$\pm$0.4} & 58.8{\scriptsize$\pm$0.0} & 0.0{\scriptsize$\pm$0.0} & 26.1{\scriptsize$\pm$0.1} \\
\midrule
\multirow{5}{*}{RAG}
  & Qwen3-0.6B     & 47.5{\scriptsize$\pm$2.3} & 27.8{\scriptsize$\pm$0.6} & 35.1{\scriptsize$\pm$0.6} & 6.4{\scriptsize$\pm$1.4} & 17.1{\scriptsize$\pm$0.6} & 0.0{\scriptsize$\pm$0.0} & 22.3{\scriptsize$\pm$0.6} \\

  & Llama-3.2-3B   & 61.6{\scriptsize$\pm$1.8} & 37.9{\scriptsize$\pm$2.0} & 45.6{\scriptsize$\pm$1.7} & 7.0{\scriptsize$\pm$0.4} & 36.5{\scriptsize$\pm$2.1} & 0.0{\scriptsize$\pm$0.0} & 31.4{\scriptsize$\pm$0.4} \\

  & Mistral-7B     & 62.1{\scriptsize$\pm$1.3} & 35.1{\scriptsize$\pm$2.1} & 48.9{\scriptsize$\pm$1.7} & 9.7{\scriptsize$\pm$0.8} & 38.8{\scriptsize$\pm$3.3} & 0.0{\scriptsize$\pm$0.0} & 32.4{\scriptsize$\pm$1.0} \\

  & Qwen3-8B       & 71.7{\scriptsize$\pm$0.5} & 50.3{\scriptsize$\pm$1.0} & 55.7{\scriptsize$\pm$0.6} & 7.8{\scriptsize$\pm$1.0} & 47.8{\scriptsize$\pm$0.7} & 0.0{\scriptsize$\pm$0.0} & 38.9{\scriptsize$\pm$0.2} \\

  & Qwen3-32B      & 77.8{\scriptsize$\pm$0.5} & 42.4{\scriptsize$\pm$2.7} & 61.1{\scriptsize$\pm$1.0} & 9.0{\scriptsize$\pm$0.4} & 52.5{\scriptsize$\pm$0.3} & 0.0{\scriptsize$\pm$0.0} & 40.5{\scriptsize$\pm$0.3} \\
\midrule
\multirow{5}{*}{Memobase}
  & Qwen3-0.6B     & 47.6{\scriptsize$\pm$1.9} & 12.6{\scriptsize$\pm$1.2} & 27.8{\scriptsize$\pm$1.9} & 3.9{\scriptsize$\pm$0.9} & 9.2{\scriptsize$\pm$3.4} & 5.4{\scriptsize$\pm$5.3} & 17.8{\scriptsize$\pm$0.7} \\

  & Llama-3.2-3B   & 50.2{\scriptsize$\pm$1.3} & 4.5{\scriptsize$\pm$1.4} & 25.0{\scriptsize$\pm$1.1} & 1.5{\scriptsize$\pm$0.6} & 30.6{\scriptsize$\pm$1.8} & 0.0{\scriptsize$\pm$0.0} & 18.6{\scriptsize$\pm$0.7} \\

  & Mistral-7B     & 54.9{\scriptsize$\pm$0.3} & 4.1{\scriptsize$\pm$2.0} & 29.5{\scriptsize$\pm$0.9} & 6.7{\scriptsize$\pm$0.6} & 44.3{\scriptsize$\pm$1.8} & 0.0{\scriptsize$\pm$0.0} & 23.3{\scriptsize$\pm$0.2} \\

  & Qwen3-8B       & 65.8{\scriptsize$\pm$1.2} & 2.6{\scriptsize$\pm$0.3} & 30.4{\scriptsize$\pm$0.5} & 4.3{\scriptsize$\pm$0.7} & 41.0{\scriptsize$\pm$0.7} & 0.0{\scriptsize$\pm$0.0} & 24.0{\scriptsize$\pm$0.3} \\

  & Qwen3-32B      & 73.1{\scriptsize$\pm$1.6} & 1.8{\scriptsize$\pm$1.0} & 23.4{\scriptsize$\pm$2.0} & 5.1{\scriptsize$\pm$2.2} & 33.7{\scriptsize$\pm$1.8} & 18.9{\scriptsize$\pm$32.8} & 26.0{\scriptsize$\pm$6.1} \\
\midrule
\multirow{5}{*}{MemSearch}
  & Qwen3-0.6B     & 77.8{\scriptsize$\pm$0.5} & 23.1{\scriptsize$\pm$2.1} & 39.7{\scriptsize$\pm$0.9} & 5.3{\scriptsize$\pm$1.0} & 10.2{\scriptsize$\pm$0.3} & 0.0{\scriptsize$\pm$0.0} & 26.0{\scriptsize$\pm$0.5} \\

  & Llama-3.2-3B   & 80.6{\scriptsize$\pm$1.3} & 22.1{\scriptsize$\pm$3.6} & 51.7{\scriptsize$\pm$0.8} & 7.7{\scriptsize$\pm$0.9} & 33.3{\scriptsize$\pm$3.9} & 0.0{\scriptsize$\pm$0.0} & 32.6{\scriptsize$\pm$1.4} \\

  & Mistral-7B     & 75.4{\scriptsize$\pm$1.5} & 19.3{\scriptsize$\pm$2.8} & 58.6{\scriptsize$\pm$0.7} & 14.3{\scriptsize$\pm$2.9} & 35.9{\scriptsize$\pm$3.1} & 0.0{\scriptsize$\pm$0.0} & 33.9{\scriptsize$\pm$1.0} \\

  & Qwen3-8B       & 92.1{\scriptsize$\pm$0.3} & 19.7{\scriptsize$\pm$1.8} & 62.9{\scriptsize$\pm$0.9} & 8.8{\scriptsize$\pm$0.9} & 44.3{\scriptsize$\pm$0.9} & 0.9{\scriptsize$\pm$1.6} & 38.1{\scriptsize$\pm$0.2} \\

  & Qwen3-32B      & 93.3{\scriptsize$\pm$0.3} & 26.0{\scriptsize$\pm$1.8} & 69.0{\scriptsize$\pm$0.6} & 10.8{\scriptsize$\pm$2.1} & 41.4{\scriptsize$\pm$1.9} & 0.0{\scriptsize$\pm$0.0} & 40.1{\scriptsize$\pm$0.1} \\
\midrule
\multirow{5}{*}{Oracle}
  & Qwen3-0.6B     & 78.3{\scriptsize$\pm$0.9} & 35.7{\scriptsize$\pm$0.7} & 32.8{\scriptsize$\pm$0.9} & 13.7{\scriptsize$\pm$2.4} & 62.4{\scriptsize$\pm$0.0} & 39.1{\scriptsize$\pm$5.0} & 43.7{\scriptsize$\pm$0.9} \\

  & Llama-3.2-3B   & 90.6{\scriptsize$\pm$0.6} & 46.0{\scriptsize$\pm$0.3} & 64.2{\scriptsize$\pm$0.1} & 26.6{\scriptsize$\pm$1.2} & 66.9{\scriptsize$\pm$1.8} & 6.2{\scriptsize$\pm$1.5} & 50.1{\scriptsize$\pm$0.5} \\

  & Mistral-7B     & 88.4{\scriptsize$\pm$0.5} & 52.1{\scriptsize$\pm$0.6} & 71.1{\scriptsize$\pm$0.3} & 27.5{\scriptsize$\pm$0.8} & 78.4{\scriptsize$\pm$0.9} & 1.8{\scriptsize$\pm$3.1} & 53.2{\scriptsize$\pm$0.5} \\

  & Qwen3-8B       & 97.0{\scriptsize$\pm$0.0} & 55.0{\scriptsize$\pm$1.0} & 71.2{\scriptsize$\pm$0.9} & 39.9{\scriptsize$\pm$1.0} & 74.7{\scriptsize$\pm$0.6} & 11.1{\scriptsize$\pm$5.5} & 58.1{\scriptsize$\pm$1.1} \\

  & Qwen3-32B      & 97.3{\scriptsize$\pm$0.3} & 52.9{\scriptsize$\pm$1.8} & 80.9{\scriptsize$\pm$1.2} & 54.0{\scriptsize$\pm$0.7} & 78.4{\scriptsize$\pm$0.9} & 4.5{\scriptsize$\pm$1.5} & 61.3{\scriptsize$\pm$0.2} \\
