# Supplementary material for: MemArena: An Ego-Centric Benchmark for On-Device Agentic Personal Memory Assistants at Scale
Source: arXiv:2608.02613 source file (2026-10-02)
Supplement: Supplementary file 2 [file appendix_L_privacy_body.tex]

\multirow{5}{*}{Vanilla}
  & Qwen3-0.6B     & 96.8{\scriptsize$\pm$2.1} & 0.0{\scriptsize$\pm$0.0} & 23.5{\scriptsize$\pm$9.1} & 0.0{\scriptsize$\pm$0.0} \\

  & Llama-3.2-3B   & 100.0{\scriptsize$\pm$0.0} & 0.0{\scriptsize$\pm$0.0} & 51.2{\scriptsize$\pm$1.6} & 0.0{\scriptsize$\pm$0.0} \\

  & Mistral-7B     & 99.5{\scriptsize$\pm$0.8} & 0.0{\scriptsize$\pm$0.0} & 44.1{\scriptsize$\pm$2.9} & 0.0{\scriptsize$\pm$0.0} \\

  & Qwen3-8B       & 100.0{\scriptsize$\pm$0.0} & 0.0{\scriptsize$\pm$0.0} & 55.4{\scriptsize$\pm$4.5} & 0.0{\scriptsize$\pm$0.0} \\

  & Qwen3-32B      & 100.0{\scriptsize$\pm$0.0} & 0.0{\scriptsize$\pm$0.0} & 47.4{\scriptsize$\pm$2.2} & 0.0{\scriptsize$\pm$0.0} \\
\midrule
\multirow{5}{*}{RAG}
  & Qwen3-0.6B     & 96.3{\scriptsize$\pm$1.6} & 0.0{\scriptsize$\pm$0.0} & 36.6{\scriptsize$\pm$4.9} & 0.0{\scriptsize$\pm$0.0} \\

  & Llama-3.2-3B   & 87.2{\scriptsize$\pm$0.8} & 0.0{\scriptsize$\pm$0.0} & 30.0{\scriptsize$\pm$2.9} & 0.0{\scriptsize$\pm$0.0} \\

  & Mistral-7B     & 87.7{\scriptsize$\pm$1.4} & 0.0{\scriptsize$\pm$0.0} & 55.9{\scriptsize$\pm$2.2} & 0.0{\scriptsize$\pm$0.0} \\

  & Qwen3-8B       & 81.3{\scriptsize$\pm$0.8} & 0.0{\scriptsize$\pm$0.0} & 49.8{\scriptsize$\pm$2.9} & 0.0{\scriptsize$\pm$0.0} \\

  & Qwen3-32B      & 81.3{\scriptsize$\pm$0.8} & 0.0{\scriptsize$\pm$0.0} & 53.1{\scriptsize$\pm$5.7} & 0.0{\scriptsize$\pm$0.0} \\
\midrule
\multirow{5}{*}{Memobase}
  & Qwen3-0.6B     & 100.0{\scriptsize$\pm$0.0} & 2.8{\scriptsize$\pm$2.8} & 44.6{\scriptsize$\pm$9.4} & 5.4{\scriptsize$\pm$5.3} \\

  & Llama-3.2-3B   & 100.0{\scriptsize$\pm$0.0} & 0.0{\scriptsize$\pm$0.0} & 50.2{\scriptsize$\pm$9.4} & 0.0{\scriptsize$\pm$0.0} \\

  & Mistral-7B     & 89.0{\scriptsize$\pm$9.0} & 0.0{\scriptsize$\pm$0.0} & 47.9{\scriptsize$\pm$2.8} & 0.0{\scriptsize$\pm$0.0} \\

  & Qwen3-8B       & 98.2{\scriptsize$\pm$1.6} & 0.0{\scriptsize$\pm$0.0} & 45.1{\scriptsize$\pm$16.0} & 0.0{\scriptsize$\pm$0.0} \\

  & Qwen3-32B      & 95.4{\scriptsize$\pm$7.9} & 14.1{\scriptsize$\pm$24.4} & 37.1{\scriptsize$\pm$20.8} & 18.9{\scriptsize$\pm$32.8} \\
\midrule
\multirow{5}{*}{MemSearch}
  & Qwen3-0.6B     & 98.2{\scriptsize$\pm$0.8} & 0.0{\scriptsize$\pm$0.0} & 32.9{\scriptsize$\pm$4.5} & 0.0{\scriptsize$\pm$0.0} \\

  & Llama-3.2-3B   & 95.9{\scriptsize$\pm$0.0} & 0.0{\scriptsize$\pm$0.0} & 30.5{\scriptsize$\pm$2.9} & 0.0{\scriptsize$\pm$0.0} \\

  & Mistral-7B     & 94.5{\scriptsize$\pm$1.4} & 0.0{\scriptsize$\pm$0.0} & 56.3{\scriptsize$\pm$2.4} & 0.0{\scriptsize$\pm$0.0} \\

  & Qwen3-8B       & 90.9{\scriptsize$\pm$1.6} & 0.5{\scriptsize$\pm$0.8} & 45.5{\scriptsize$\pm$4.5} & 0.9{\scriptsize$\pm$1.6} \\

  & Qwen3-32B      & 89.0{\scriptsize$\pm$0.0} & 0.0{\scriptsize$\pm$0.0} & 44.1{\scriptsize$\pm$2.9} & 0.0{\scriptsize$\pm$0.0} \\
\midrule
\multirow{5}{*}{Oracle}
  & Qwen3-0.6B     & 25.1{\scriptsize$\pm$4.0} & 89.2{\scriptsize$\pm$2.2} & 2.8{\scriptsize$\pm$0.0} & 39.1{\scriptsize$\pm$5.0} \\

  & Llama-3.2-3B   & 3.2{\scriptsize$\pm$0.8} & 98.1{\scriptsize$\pm$3.3} & 1.9{\scriptsize$\pm$3.3} & 6.2{\scriptsize$\pm$1.5} \\

  & Mistral-7B     & 0.9{\scriptsize$\pm$1.6} & 100.0{\scriptsize$\pm$0.0} & 0.0{\scriptsize$\pm$0.0} & 1.8{\scriptsize$\pm$3.1} \\

  & Qwen3-8B       & 5.9{\scriptsize$\pm$3.2} & 100.0{\scriptsize$\pm$0.0} & 0.0{\scriptsize$\pm$0.0} & 11.1{\scriptsize$\pm$5.5} \\

  & Qwen3-32B      & 2.3{\scriptsize$\pm$0.8} & 98.6{\scriptsize$\pm$1.4} & 1.4{\scriptsize$\pm$1.4} & 4.5{\scriptsize$\pm$1.5} \\
