# Supplementary material for: MemArena: An Ego-Centric Benchmark for On-Device Agentic Personal Memory Assistants at Scale
Source: arXiv:2608.02613 source file (2026-10-02)
Supplement: Supplementary file 3 [file appendix_access_markers_body.tex]

Qwen3-0.6B    & $39.1$ & $43.8$ & $+4.7$ & $[-1.3,\ +8.3]$ \\
Llama-3.2-3B  & $6.2$ & $7.0$ & $+0.8$ & $[0.0,\ +2.5]$ \\
Mistral-7B    & $1.8$ & $1.8$ & $0.0$ & $[-2.6,\ +2.7]$ \\
Qwen3-8B      & $11.1$ & $15.2$ & $+4.1$ & $[-2.3,\ +7.3]$ \\
Qwen3-32B-AWQ & $4.5$ & $3.6$ & $-0.9$ & $[-5.3,\ +2.6]$ \\
\midrule
Mean ($15$ cells) & $12.5$ & $14.3$ & $+1.7$ & $[-5.3,\ +8.3]$ \\
