# Supplementary material for: MemArena: An Ego-Centric Benchmark for On-Device Agentic Personal Memory Assistants at Scale
Source: arXiv:2608.02613 source file (2026-10-02)
Supplement: Supplementary file 4 [file appendix_cross_extractor_writer32_body.tex]

\multirow{4}{*}{Memobase}
  & Qwen3-0.6B   & $47.6${\scriptsize$\pm1.9$} & $12.6${\scriptsize$\pm1.2$} & $27.8${\scriptsize$\pm1.9$} & $\phantom{0}3.9${\scriptsize$\pm0.9$} & $\phantom{0}9.2${\scriptsize$\pm3.4$} & $\phantom{0}5.4${\scriptsize$\pm5.3$} & $17.8${\scriptsize$\pm0.7$} \\
  & Llama-3.2-3B & $50.2${\scriptsize$\pm1.3$} & $\phantom{0}4.5${\scriptsize$\pm1.4$} & $25.0${\scriptsize$\pm1.1$} & $\phantom{0}1.5${\scriptsize$\pm0.6$} & $30.6${\scriptsize$\pm1.8$} & $\phantom{0}0.0${\scriptsize$\pm0.0$} & $18.6${\scriptsize$\pm0.7$} \\
  & Mistral-7B   & $54.9${\scriptsize$\pm0.3$} & $\phantom{0}4.1${\scriptsize$\pm2.0$} & $29.5${\scriptsize$\pm0.9$} & $\phantom{0}6.7${\scriptsize$\pm0.6$} & $44.3${\scriptsize$\pm1.8$} & $\phantom{0}0.0${\scriptsize$\pm0.0$} & $23.3${\scriptsize$\pm0.2$} \\
  & Qwen3-8B     & $65.8${\scriptsize$\pm1.2$} & $\phantom{0}2.6${\scriptsize$\pm0.3$} & $30.4${\scriptsize$\pm0.5$} & $\phantom{0}4.3${\scriptsize$\pm0.7$} & $41.0${\scriptsize$\pm0.7$} & $\phantom{0}0.0${\scriptsize$\pm0.0$} & $24.0${\scriptsize$\pm0.3$} \\
\midrule
\multirow{4}{*}{Memobase-writer32}
  & Qwen3-0.6B   & $50.5${\scriptsize$\pm0.9$} & $14.6${\scriptsize$\pm0.7$} & $30.4${\scriptsize$\pm1.0$} & $\phantom{0}3.4${\scriptsize$\pm0.6$} & $\phantom{0}6.7${\scriptsize$\pm0.9$} & $18.3${\scriptsize$\pm27.1$} & $20.7${\scriptsize$\pm4.5$} \\
  & Llama-3.2-3B & $57.1${\scriptsize$\pm0.5$} & $\phantom{0}3.4${\scriptsize$\pm0.7$} & $26.6${\scriptsize$\pm1.3$} & $\phantom{0}2.2${\scriptsize$\pm0.9$} & $26.1${\scriptsize$\pm0.3$} & $18.9${\scriptsize$\pm32.8$} & $22.4${\scriptsize$\pm5.5$} \\
  & Mistral-7B   & $56.2${\scriptsize$\pm0.6$} & $\phantom{0}3.4${\scriptsize$\pm0.9$} & $28.6${\scriptsize$\pm0.6$} & $\phantom{0}7.9${\scriptsize$\pm2.1$} & $39.0${\scriptsize$\pm2.4$} & $19.8${\scriptsize$\pm32.0$} & $25.8${\scriptsize$\pm5.6$} \\
  & Qwen3-8B     & $67.2${\scriptsize$\pm1.5$} & $\phantom{0}3.6${\scriptsize$\pm0.6$} & $31.8${\scriptsize$\pm0.8$} & $\phantom{0}2.7${\scriptsize$\pm0.9$} & $40.4${\scriptsize$\pm3.2$} & $17.2${\scriptsize$\pm29.8$} & $27.1${\scriptsize$\pm5.0$} \\
