# Supplementary material for: MemArena: An Ego-Centric Benchmark for On-Device Agentic Personal Memory Assistants at Scale
Source: arXiv:2608.02613 source file (2026-10-02)
Supplement: Supplementary file 5 [file appendix_cross_family_body.tex]

\multirow{2}{*}{Vanilla}
  & Llama-3.2-3B   & 58.6{\scriptsize$\pm$2.3} & 3.2{\scriptsize$\pm$0.3} & 27.8{\scriptsize$\pm$0.2} & 2.9{\scriptsize$\pm$0.8} & 58.4{\scriptsize$\pm$0.3} & 0.0{\scriptsize$\pm$0.0} & 25.2{\scriptsize$\pm$0.3} \\

  & Mistral-7B     & 54.7{\scriptsize$\pm$0.6} & 2.2{\scriptsize$\pm$0.3} & 37.3{\scriptsize$\pm$0.8} & 3.2{\scriptsize$\pm$0.3} & 56.7{\scriptsize$\pm$0.3} & 0.0{\scriptsize$\pm$0.0} & 25.7{\scriptsize$\pm$0.1} \\
\midrule
\multirow{2}{*}{RAG}
  & Llama-3.2-3B   & 61.6{\scriptsize$\pm$1.8} & 37.9{\scriptsize$\pm$2.0} & 45.6{\scriptsize$\pm$1.7} & 7.0{\scriptsize$\pm$0.4} & 36.5{\scriptsize$\pm$2.1} & 0.0{\scriptsize$\pm$0.0} & 31.4{\scriptsize$\pm$0.4} \\

  & Mistral-7B     & 62.1{\scriptsize$\pm$1.3} & 35.1{\scriptsize$\pm$2.1} & 48.9{\scriptsize$\pm$1.7} & 9.7{\scriptsize$\pm$0.8} & 38.8{\scriptsize$\pm$3.3} & 0.0{\scriptsize$\pm$0.0} & 32.4{\scriptsize$\pm$1.0} \\
\midrule
\multirow{2}{*}{Memobase}
  & Llama-3.2-3B   & 50.2{\scriptsize$\pm$1.3} & 4.5{\scriptsize$\pm$1.4} & 25.0{\scriptsize$\pm$1.1} & 1.5{\scriptsize$\pm$0.6} & 30.6{\scriptsize$\pm$1.8} & 0.0{\scriptsize$\pm$0.0} & 18.6{\scriptsize$\pm$0.7} \\

  & Mistral-7B     & 54.9{\scriptsize$\pm$0.3} & 4.1{\scriptsize$\pm$2.0} & 29.5{\scriptsize$\pm$0.9} & 6.7{\scriptsize$\pm$0.6} & 44.3{\scriptsize$\pm$1.8} & 0.0{\scriptsize$\pm$0.0} & 23.3{\scriptsize$\pm$0.2} \\
\midrule
\multirow{2}{*}{MemSearch}
  & Llama-3.2-3B   & 80.6{\scriptsize$\pm$1.3} & 22.1{\scriptsize$\pm$3.6} & 51.7{\scriptsize$\pm$0.8} & 7.7{\scriptsize$\pm$0.9} & 33.3{\scriptsize$\pm$3.9} & 0.0{\scriptsize$\pm$0.0} & 32.6{\scriptsize$\pm$1.4} \\

  & Mistral-7B     & 75.4{\scriptsize$\pm$1.5} & 19.3{\scriptsize$\pm$2.8} & 58.6{\scriptsize$\pm$0.7} & 14.3{\scriptsize$\pm$2.9} & 35.9{\scriptsize$\pm$3.1} & 0.0{\scriptsize$\pm$0.0} & 33.9{\scriptsize$\pm$1.0} \\
\midrule
\multirow{2}{*}{Oracle}
  & Llama-3.2-3B   & 90.6{\scriptsize$\pm$0.6} & 46.0{\scriptsize$\pm$0.3} & 64.2{\scriptsize$\pm$0.1} & 26.6{\scriptsize$\pm$1.2} & 66.9{\scriptsize$\pm$1.8} & 6.2{\scriptsize$\pm$1.5} & 50.1{\scriptsize$\pm$0.5} \\

  & Mistral-7B     & 88.4{\scriptsize$\pm$0.5} & 52.1{\scriptsize$\pm$0.6} & 71.1{\scriptsize$\pm$0.3} & 27.5{\scriptsize$\pm$0.8} & 78.4{\scriptsize$\pm$0.9} & 1.8{\scriptsize$\pm$3.1} & 53.2{\scriptsize$\pm$0.5} \\
