# Supplementary material for: MemArena: An Ego-Centric Benchmark for On-Device Agentic Personal Memory Assistants at Scale
Source: arXiv:2608.02613 source file (2026-10-02)
Supplement: Supplementary file 6 [file appendix_latency_fit_body.tex]

Qwen3-0.6B & 12.9 & 23.7 & 1.24 & 0.9992 & 4.3 & 18.9 & 7.8 & 0.50 \\
Llama-3.2-3B & 50.2 & 83.0 & 1.82 & 0.9995 & 1.7 & 6.8 & 36.1 & 0.53 \\
Mistral-7B-Inst.\ v0.3 & -- & -- & -- & -- & -- & -- & -- & -- \\
Qwen3-8B & 127.0 & 205.6 & 2.73 & 0.9984 & 2.6 & 17.2 & 71.3 & 0.63 \\
Qwen3-32B-AWQ & 188.5 & 959.0 & 14.40 & 0.9984 & 3.2 & 27.2 & 80.6 & 1.11 \\
