# Supplementary material for: MemArena: An Ego-Centric Benchmark for On-Device Agentic Personal Memory Assistants at Scale
Source: arXiv:2608.02613 source file (2026-10-02)
Supplement: Supplementary file 7 [file appendix_latency_predicted_body.tex]

Qwen3-0.6B & 394 & 260 & 654 & 480 & 874 \\
Llama-3.2-3B & 1410 & 1121 & 1643 & 1884 & 3060 \\
Mistral-7B-Inst.\ v0.3 & \texttt{n/a} & \texttt{n/a} & \texttt{n/a} & \texttt{n/a} & \texttt{n/a} \\
Qwen3-8B & 2150 & 2402 & 4636 & 3799 & 6072 \\
Qwen3-32B-AWQ & 7247 & 4549 & 7173 & 6147 & 10853 \\
\midrule
$T_{\text{search}}$ (ms, p50) & 0 & 0 & 87 & 8 & 51 \\
